# Supplementary material for: Can Contrastive Learning Refine Embeddings
Source: arXiv:2404.08701 source file (2024-04-11)
Supplement: Supplementary file 1 [file 009_appendix.tex]

\subsection{Notations}
The notation used in this paper is summarized in Table ~\ref{notation} for easy reference. 

\begin{table}[h]
	\centering
	\caption{Notations and definitions }
	\setlength\tabcolsep{1.5pt} % default value: 6pt
	\begin{tabular}{|c|c|}
		\hline
		{\bf Symbols}       & {\bf Definition}                \\ \hline
  D & dataset  \\ \hline
  $d_i$ & the $i$th data point  \\ \hline
  h() & the embedding function  \\ \hline
  $\mathcal{X}$ & the dataset embedding  \\ \hline
  f() & the contrastive encoder  \\ \hline
  %g() & the contrastive learning architecture  \\ \hline
  F & the function space  \\ \hline
  T & the downstream task  \\ \hline
  %$\mathcal{X}$ & the input data points \\ \hline
  $l()$ & the loss function  \\ \hline
  L & the total loss  \\ \hline
	\end{tabular}
\label{notation}
\end{table}

\subsection{Theoretical Proof}
\noindent{\bf A - Preliminary.}
We first set up notation and describe the framework for standard deep nueral networks (DNNs) and skip connection based neural network  that will be essential for our analysis. 
Let $\mathcal{X}$ denote the set of all possible data points,
traditionally, a simple multi-layer neural network (MLP) can be denoted as 
\begin{align}
f_1(x) = \Pi_{l=1}^L W^l x
\end{align}
where $W^l$ is the model parameter of the $l$th layer. A neural network with skip connection for very two layers can be denoted as 
\begin{align}
f_2(x) = \Pi_{l=1}^{L/2} (W^{2l}W^{2l-1} + \mathrm{I}) x
\end{align}
Note that $f_1$ and $f_2$ have the same amount of layers.

Suppose we have a neural network $f_I(x) = \Pi_{l=1}^L \mathrm{I} x$ where $\mathrm{I}$ is the identity matrix.
In this way, we can write the network with skip connection as
\begin{align}\label{res_formula}
f_2(x) = f_I + f_1(x)
\end{align}

\noindent{\bf B - Downstream Task Loss for Contrastive Unsupervised Learning.}
In this section, we provide a theoretical proof for how skip connections in contrastive learning can improve the robustness of embeddings. The proof is divided into two parts. First, we present an upper bound for the loss of a supervised downstream task in any contrastive learning, as originally shown in ~\cite{bound}. We then show that using skip connections in contrastive learning can decrease or maintain this upper bound for downstream tasks.

% In unsupervised learning, the primary objective is typically to minimize the following loss function
% \begin{align}
% E [-log (\frac{e^{f(x)^T f(x^+)}}{e^{f(x)^T f(x^+)} + e^{f(x)^T f(x^-)}})]
% \end{align}
% where $(x, x^+)$ is a pair of similar data points and $x^-$ is a data point that is dissimilar to $x$ (often chosen at random) and is referred to as a negative sample.
% The purpose of this loss function is to ensure that the embeddings of the positive pair, generated by the function $f()$, are similar to each other, while the embeddings of the negative pair, generated by the same function, are dissimilar to each other.

Contrastive learning assumes access to similar data in the form of pairs ($x$, $x^+$) that come from a distribution $\mathcal{X}$ as well as $k$ i.i.d. negative samples $x_1^-, x_2^-, ..., x_k^-$ from a distribution $\mathcal{X}_{neg}$ that are presumably unrelated to $x$. 
Learning is done over $\mathcal{F}$, a class of representation functions $f: \mathcal{X} \longrightarrow R^d$, $f$ is the embedding function. 
The quality of the representation function $f$ (contrastive encoder) is evaluated by its performance on a multi-class classification task $\mathrm{T} \in \mathcal{T}$ using linear classification. 
A multi-class classifier for $\mathrm{T} \in \mathcal{T}$ is a function $g$  whose output coordinates are indexed by the classes $c$ in task $\mathrm{T} \in \mathcal{T}$.
In SimCLR ~\cite{simCLR}, $g(x) = w f(x)$. 
The two losses considered in ~\cite{bound} are the standard hinge loss $l(v) = \textrm{max}\{0; 1 + \textrm{max}_i \{- v_i \} \}$ and the logistic loss $l(v) = \textrm(log)_2 (1 + \sum_i \textrm{exp} (- v_i))$ for $v \in R^k$. Then the supervised loss of the downstream task classifier $g$ is 
\begin{align}
    L_{sup}(\mathbf{T}, g) = E [l( \{g(x)_c - g(x)_{c'} \}_{c \neq c'})]
\end{align}
For simplicity, we use $L_{sup}(f)$ to denote the downstream loss of the model with function $f()$ which satisfies $L_{sup}(\mathbf{T}, g)$ and $g(x) = w f(x)$.

We outline the objective of contrastive learning: $k$ denotes number of negative samples used for training.
The unsurpervise loss can be defined as 
\begin{align}
    L_{un}(f) = E[l(\{f(x)^T (f(x^+) - f(x^-)\}_{i=1}^k)]
\end{align}
After training, suppose $\hat{f}$ is the function which can minimizes the empirical unsupervised loss
and we denote its corresponding loss for supervised downstream task as $L_{sup}(\hat{f})$.
According to the theorim 4.1 in ~\cite{bound}, we have
\begin{align}\label{upper_bond}
    L_{sup}(\hat{f}) <= \alpha L_{un}(f) + \eta Gen_M + \epsilon
\end{align}

where $Gen$ is the generalization error which is defined as 
\begin{align}
Gen_M = O(R \sqrt{k} \frac{R_s (F)}{M} + (R^2 + log k) \sqrt{\frac{log \frac{1}{\epsilon}}{M}}
\end{align}
and $M$ is the sample size, $R_s (F)$ is the Rademacher average of $F$.

\begin{figure}
    \centering
    \includegraphics[width=0.3\textwidth]{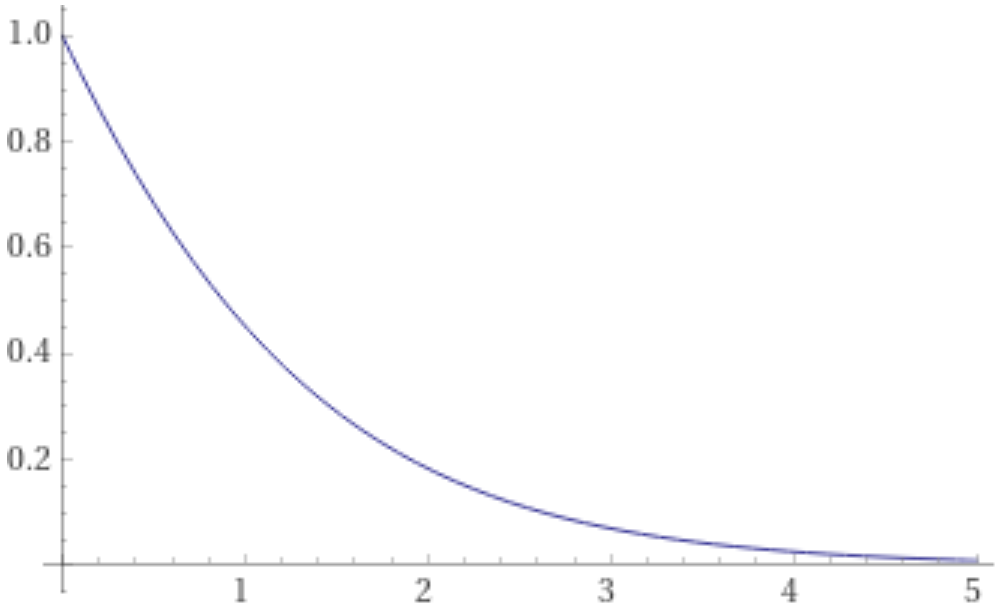}
    \caption{The logistic loss.}
    \label{logistic_loss}
\end{figure}

\noindent{\bf C - Skip-connection Based Model.}
Suppose we use neural network with skip connection to learn the contrastive embedding, according to Eq.~\eqref{res_formula}, we have 
\begin{align*}
L_{un}(f) &= E[l(\{f_2(x)^T (f_2(x^+) - f_2(x^-)\}_{i=1}^k)] \\
& = E[l(\{(f_I(x) + f_1(x))^T (f_I(x^+) + f_1(x^+) \\
&- f_I(x^-) - f_1(x^-)\}_{i=1}^k)] \\
\end{align*}
where $l()$ is the logistic loss, as illustrated in Figure ~\ref{logistic_loss}.
If we assume that the weights for $f_1(x)$ are also identity matrix $\mathrm{I}$ and $f_I(x)^T (f_I(x^+) - f_I(x^-)) >= 0$ which is a typical instance, we can have
\begin{align*}
L_{un}(f) &= E[l(4 \{f_I(x)^T (f_I(x^+) - f_I(x^-)\}_{i=1}^k)] \\
& <= E[l(\{f_I(x)^T (f_I(x^+) - f_I(x^-)\}_{i=1}^k)]
\end{align*}
which means the upper bond of resnet is smaller than $f_I$.
When the weights for $f_1(x)$ are not identity matrix,
according to the universal approximation theory of deep neural network, 
$L_{un}(f)$ should be smaller or equal than $L_{un}(f_I)$.

The identity MLP, $f(x) = \mathbf{I} \mathbf{I} \mathbf{I} \mathbf{I} x = x$, is a special case of an MLP. 
Bring it to Eq.~\eqref{upper_bond}, 
This implies that the loss of a ResNet should not be greater than that of the identity MLP. Therefore, the upper bound for using skip connections for learning should be lower.

\subsection{Datasets}

\begin{itemize}
  \item The \textbf{movieQA} dataset is composed of a movie ontology derived from the WikiMovies Dataset. It includes over 40,000 triples that provide information about movies.
  \item The \textbf{STL10} dataset is used for developing unsupervised feature learning, deep learning, and self-taught learning algorithms. It contains both labeled and unlabeled images, with the labeled images belonging to 10 classes.
  \item The \textbf{CIFAR10} dataset includes 60000 32x32 color images in 10 classes, with 6000 images per class. The dataset is split into 50000 training images and 10000 test images.
  \item The \textbf{Cora} dataset is a graph data consisting of 2708 scientific publications classified into one of seven classes. The citation network is composed of 5429 links.
  \item The \textbf{Pubmed} dataset is a graph data containing citations and abstracts of biomedical literature from various NLM literature resources.
\end{itemize}

\subsection{Base Methods}

\begin{itemize}
    \item FedE ~\cite{fedE} is a Federated Knowledge Graph Embedding framework that focuses on learning knowledge graph embeddings by aggregating locally-computed updates. This framework includes a client for each knowledge graph and a server for coordinating embedding aggregation.
    \item SimCLR ~\cite{simCLR} is a simple framework for contrastive learning of visual representations. It first learns generic representations of images on an unlabeled dataset and then can be fine-tuned with a small number of labeled images to achieve good performance for a given classification task.
    \item GraphSAGE ~\cite{graphsage} is a general, inductive framework that leverages node feature information (e.g., text attributes) to efficiently generate node embeddings.
\end{itemize}

\subsection{Downstream Task Details}
The third downstream task for federated learning is movie recommendation which recommends new movies to users according to the user's watching history where the data is from Netflix dataset  \url{https://www.kaggle.com/code/laowingkin/netflix-movie-recommendation/data}. Given a user's watching history $V_1, ..., V_N$, we treat $V_1, .., V_{N-10}$ as the training data, and predict 10 movies the user is most likely to watch. Then, we calculate how many movies in the 10 predicted movies belong to $V_{N-9}, ..., V_N$.
